# Supplementary material for: An Exploratory Analysis of Biased Learners in Soft-Sensing Frames
Source: arXiv:1904.10753 ancillary file (2019-04-24)
Supplement: Supplementary file 1 [file supp.pdf]

# Supplementary Material

# An Exploratory Analysis of Biased Learners in Soft-Sensing Frames

**Aysun Urhan[§a], Burak Alakent[§b]**

[§]: Department of Chemical Engineering, Bogazici University, Bebek, Istanbul, 34342, Turkey

Declarations of interest: None.

[a]: aysun.urhan@boun.edu.tr

[b]: burak.alakent@boun.edu.tr

## Text S1. CSTR Simulation details

Reactant, and solvent streams, denoted as $F_A$ and $F_S$, respectively, enter the reactor, in which temperature controller manipulates the coolant flowrate $F_C$, and the reactor height is controlled with a level controller, which sets the reactor effluent flowrate, $F_{out}$. Temperature of the solvent entering the reactor is controlled by manipulating the flowrate of the jacket fluid, and the liquid height inside the heater is controlled with a level controller (Fig. S1).

Simulation variables are considered in two groups, which correspond to two processes, the heater and the reactor; accordingly, the subscripts hex and reactor are used to differentiate these groups of variables from one another, unless the variable contributes to both processes directly. Let TC and LC denote temperature and level controllers in the reactor unit, with $TC_{hex}$ and $FC_{hex}$ being the equivalent controllers for the heating unit; the subscript sp stands for the controller set point, drawn with dashed lines in Fig. S1. Reactor was modeled with the following material and energy balances from Yoon and MacGregor [1]:

$$\frac{dC_A}{dt} = \frac{F}{V}C_{A0} - \frac{F}{V}C_A - k_0 e^{-\frac{E}{RT}}C_A$$

$$V\rho_L C_{p,L}\frac{dT}{dt} = \rho_L C_{p,L}F(T_0 - T) - \frac{aF_C^{b+1}}{F_C + aF_C^{b}/2\rho_L C_{p,L}} + \left(T - T_{C,in}\right) - \Delta H_{rxn}V - k_0 e^{-\frac{E}{RT}}C_A$$

Mass and energy balance equations of the heat exchanger model are as follows:

$$q = UA\left(T_{j,out} - T_{out}\right)$$

$$\rho_S C_{p,S} V_S \frac{dT_{out}}{dt} = F_{in}(T_{in} - T_{out}) + q$$

$$\rho_j C_{p,j} V_j \frac{dT_{j,out}}{dt} = F_j\left(T_{j,in} - T_{j,out}\right) - q$$

$$A_{cont} \frac{dF_{out}}{dt} = F_{in} - F_{out}$$

$U_{hex}$, and $A_{hex}$ are heat transfer coefficient and area, respectively, while $\rho$, V, $C_p$ and F are density, volume, heat capacity and flowrate. Subscripts L, S, and j denote the process, solvent and the heating fluids, respectively. Values of simulation parameters and physical constants, controller settings and nominal operating points of process variables, are shown in Table S1, S2 and S3, respectively.

In the current simulation scenario, the aim is to predict the outlet concentration of the reactor product, $C_B$. Gaussian measurement noise with zero mean and variance $\sigma_e^2$ was added to all variables to mimic real life process measurements. In all input variables, except for the inlet concentration of A in the reactant stream, the following stochastic first order autoregressive (AR) model is used to imitate virtual drift:

$$u_t = \phi_u u_{t-1} + a_u$$

Here, $u$ stands for input variable, and the subscripts correspond to its time stamp. $\phi$ is the AR coefficient, and $a_u$ is the random disturbance term, specific to each input. Disturbances in the controller setpoints were modeled as Bernoulli trials with success probability $p_u$ at each time $t$. AR model coefficients and other parameters of stochastic equations can be found in Table S4.

A total of 9 concept drift models (CDMs) are constructed by changing the concentration of reactant ($C_{A0}$) in the reactor inlet stream (Fig. S2). First model represents the scenario in which concept

drift is absent, whereas the final 8 models mimic different types of real concept drift that may be encountered in real life processes (Table S5).

## Supplementary References

Yoon, S., & MacGregor, J. F. (2001). Fault diagnosis with multivariate statistical models part I: Using steady state fault signatures. *Journal of Process Control*, *11*(4), 387–400. https://doi.org/10.1016/S0959-1524(00)00008-1

## Supplementary Algorithms

Algorithm S1. $\text{Check}_{\text{M}}$ subroutine.

---

**Input:** Historical database, $D = \{(\mathbf{x}_t, \mathrm{y}_t)\}_{t=1}^{N_0+k}$ with initial training set size $N_0$; current window size, W; $k^{\text{th}}$ query point $\mathbf{x}'_k$; window increment, $\delta$; significance levels $\alpha_1$ and $\alpha_2$, satisfying $\alpha_1 < \alpha_2$.

**Initialization:**

1. Compute upper bound $\text{UB}_{\alpha_1}$ using Eq. (11)

2. Compute $d_{\text{M}}^2(\mathbf{X}_{\text{MW}})$ using Eq. (10) with $\mathbf{X}_{\text{MW}} := \{(\mathbf{x}_t)\}_{t=N_0+k-\text{W}}^{N_0+k-1}$

3. Set $S_{\text{W}} = \text{W}$; set of window sizes tested; $S_d = d_{\text{M}}^2$, set of distance values corresponding to window sizes in $S_{\text{W}}$; Initialize $I_{\text{M}} = 0$, an indicator variable for the test result.

**Mahalanobis distance check:**

4. **If** $d_{\text{M}}^2(\mathbf{X}_{\text{MW}}) \leq \text{UB}_{\alpha_1}$ **then Return** W, $I_{\text{M}}$ **end if**

5. Set $I_{\text{M}} = 1$, a positive test result is obtained

6. **While** $d_{\text{M}}^2(\mathbf{X}_{\text{MW}}) > \text{UB}_{\alpha_1}$ **do**

   (a) $\text{W} \leftarrow \text{W} \times (1 + \delta)$, extend the current window to include more observations; $\mathbf{X}_{\text{MW}} := \{(\mathbf{x}_t)\}_{t=N_0+k-\text{W}}^{N_0+k-1}$;

   (b) **If** $\text{W} > N_0 + k - 1$ **then**

      i. Compute $\text{UB}_{\alpha_2}$ using Eq. (11) to relax the upper limit since W cannot exceed $N$

      ii. Initialize a new set of window sizes $S_{\text{W}}^* = \emptyset$, for the new upper limit.

      iii. **For all** $\text{W} \in S_{\text{W}}$, **if** $d_{\text{M}}^2(\mathbf{X}_{\text{MW}}) < \text{UB}_{\alpha_2}$ **then**

---

$S_{\mathrm{W}}^{*} \leftarrow S_{\mathrm{W}}^{*} \cup \{\mathrm{W}\}$, store all past window sizes satisfying the relaxed condition. **End if**.

iv. **End for**

v. $\mathrm{W} = \begin{cases} \min S_{\mathrm{W}}^{*} & \text{if } S_{\mathrm{W}}^{*} \neq \emptyset \\ \underset{\mathrm{W} \in S_{\mathrm{W}}}{\operatorname{argmin}}\, d_{\mathrm{M}}^{2}(\mathbf{X}_{\mathrm{MW}}) & \text{otherwise} \end{cases}$

vi. **Return** W, $I_{\mathrm{M}}$ **end if**

vii. Compute $d_{\mathrm{M}}^{2}(\mathbf{X}_{\mathrm{MW}})$ using Eq. (10) with $\mathbf{X}_{\mathrm{MW}} := \{(\mathbf{x}_t)\}_{t=N_0+k-\mathrm{W}}^{N_0+k-1}$; Append distance and window size to the sets $S_d \leftarrow S_d \cup \{d_{\mathrm{M}}^{2}\}$; $S_{\mathrm{W}} \leftarrow S_{\mathrm{W}} \cup \{\mathrm{W}\}$

viii. **End while**

ix. **Return** W, $I_{\mathrm{M}}$

## Supplementary Tables

Table S1. Physical constants and parameters for the CSTR simulation.

| Parameter | Description | Value |
|---|---|---|
| $A_{reactor}$ | Base area of reactor | $3m^2$ |
| $\rho_L$ | Density of the process fluid | $1\times10^6$ |
| E/R | Activation energy term | $8.3301\times10^3$ K |
| $C_{p,L}$ | Heat capacity of process fluid | 1 cal/gK |
| a | - | $1.678\times10^6$ |
| b | - | 0.5 |
| $k_0$ | Rate constant | $1\times10^{10}$ $m^3$/kmol.min |
| $\Delta H_{rxn}$ | Enthalpy of reaction | $-1.3\times10^7$ cal/kmol |
| $\rho_S$ | Density of solvent stream | $1\times10^3$ $kg/m^3$ |
| $C_{p,S}$ | Heat capacity of solvent stream | $1\times10^3$ cal/gK |
| $\rho_j$ | Density of jacket fluid | $0.83\times10^3$ $kg/m^3$ |
| $C_{p,j}$ | Heat capacity of jacket fluid | $0.5\times10^3$ cal/gK |
| $A_{cont}$ | Base area of the container | 1 $m^2$ |

Table S2. Controller settings for the CSTR simulation.

| Controller | Proportional | Integral | Range |
|---|---|---|---|
| TC | -0.3 | -0.1 | [-0.9, 9] |
| LC | -8 | -10 | [-14.5, 55] |
| $TC_{hex}$ | -0.5 | -0.1 | [-0.7, 2.2] |
| $LC_{hex}$ | -0.01 | -0.01 | [-0.85, 1.1] |

Table S3. Values of the process variables at the nominal operating point of the CSTR simulation.

| Variable | Description | Nominal Value | $\sigma_e^2$ |
|---|---|---|---|
| $F_{out, reactor}$ | Outlet flow rate | 1 $m^3$/min | $1\times10^{-4}$ |
| $h_{sp, reactor}$ | Height set point | 3 m | - |
| $h_{reactor}$ | Height | 3 m | $1\times10^{-4}$ |
| $F_C$ | Coolant flowrate | 15 $m^3$/min | $1\times10^{-2}$ |
| $T_{sp, reactor}$ | Temperature set point | 370 K | - |
| $T_{reactor}$ | Temperature | 370 K | $4\times10^{-4}$ |
| $T_C$ | Coolant temperature | 365 K | $2.5\times10^{-3}$ |
| $F_A$ | Reactant inlet flowrate | 0.1 $m^3$/min | $1\times10^{-6}$ |
| $T_A$ | Reactant inlet temperature | 370 K | $1\times10^{-2}$ |
| $F_S$ | Solvent inlet flowrate | 0.9 $m^3$/min | $2\times10^{-6}$ |
| $h_{sp, hex}$ | Height set point | 1.2 m | - |
| $h_{hex}$ | Height | 1.2 m | $5\times10^{-6}$ |
| $F_{j,in}$ | Jacket fluid flowrate | 0.77 $m^3$/min | $5\times10^{-6}$ |
| $T_{sp, hex}$ | Solvent temperature set point | 370 K | - |
| $T_S$ | Solvent temperature | 370 K | $1\times10^{-2}$ |
| $T_{j,in}$ | Jacket fluid inlet temperature | 460 K | $4\times10^{-6}$ |
| $T_{j, out}$ | Jacket fluid outlet temperature | 415 K | $4\times10^{-4}$ |
| $F_{s, hex}$ | Solvent inlet flowrate | 0.9 $m^3$/min | $4\times10^{-6}$ |
| $T_{s, hex}$ | Solvent inlet temperature | 342 K | $4\times10^{-6}$ |
| $C_B$ | Outlet product concentratin | 1.86 kmol/$m^3$ | $2.5\times10^{-5}$ |

Table S4. Parameters of the stochastic equations of the CSTR simulation.

| Input Variable | $\phi_u$ | $\sigma_u$ | $p$ |
|---|---|---|---|
| $h_{sp, reactor}$ | 0.8500 | 0.2000 | - |
| $T_{sp, reactor}$ | 0.6000 | 0.5000 | 0.9995 |
| $T_C$ | 0.9990 | 0.0100 | - |
| $F_A$ | 0.9900 | 0.0020 | - |
| $T_A$ | 0.9995 | 0.1000 | - |
| $h_{sp, hex}$ | 0.8500 | 0.0500 | 0.9990 |
| $T_{sp, hex}$ | 0.8000 | 8.5000 | 0.9995 |
| $T_{j,in}$ | 0.9990 | 0.2375 | |
| $F_{s, hex}$ | 0.9000 | 0.0190 | |
| $T_{s, hex}$ | 0.9990 | 0.2375 | |

Table S5. Real concept drift scenarios employed in CSTR simulations.

| CDM | Type of Real Concept Drift |
|---|---|
| Default | No real concept drift, $C_{A0}$ remains constant |
| $Step^L$ | Abrupt changes at multiple values of $C_{A0}$ w/ low frequency |
| $Step^H$ | Abrupt changes at multiple values of $C_{A0}$ w/ high frequency |
| $Step_2^L$ | Abrupt changes between two different values of $C_{A0}$ w/ low frequency |
| $Step_2^H$ | Abrupt changes between two different values of $C_{A0}$ w/ high frequency |
| $Ramp_{2P}^L$ | Gradual periodic changes between two different values of $C_{A0}$ |
| $Ramp_2^L$ | Gradual changes between two different values of $C_{A0}$ with w/ low frequency |
| $Ramp_2^H$ | Gradual changes between two different values of $C_{A0}$ with w/ high frequency |
| $Step\_Ramp_2^H$ | Gradual changes mixed with abrupt shifts in value of $C_{A0}$ w/ high frequency |

Table S6. Reported prediction results on real datasets from the literature.

| Name[i] | From the Literature | | Our Results[ii] | | | |
|---|---|---|---|---|---|---|
| | Method | RMSE | MW | | JITL | |
| | | | W | $PLS^{TS}_{MW}$/ $Lasso^{TS}_{MW}$ / $RVM_{MW}$ | \|NN\| | $PLS^{TS}_{MW}$/ $Lasso^{TS}_{MW}$ / $RVM_{MW}$ |
| DS1 | An MLP[3] | 0.030 | 50 | 0.027/0.024/0.024 | 50 | 0.023/0.020/0.021 |
| | | 0.020 | 300/300/50 | 0.026/0.025/0.024 | 50 | 0.025/0.024/0.023 |
| DS2 | LWKPCR[17] | 0.058 | 10 ($n$ = 0) | 0.0317/0.0310/0.0310 | 120 ($n$ = 12) | 0.0366/0.0352/0.0394 |
| DS3 | NUFCA[76] | 0.024 | 30 | 0.0194/0.0181/0.0190 | 20/30/30 | 0.0219/0.0216/0.0219 |
| DS4 | JLSSVR[25] | - | 70/50/50 | 65.9/60.2/63.5 | 70/60/60 | 65.5/60.9/62.1 |
| | | 0.849 | 70 | 1.60/1.68/2.21 | 70/60/60 | 1.62/1.57/1.84 |
| | | 0.033 | 40/50/40 | 0.065/0.053/0.060 | 70/70/40 | 0.091/0.061/0.077 |
| DS5 | ALSSVR[70] | 1.2 | 40 | 1.43/1.42/1.43 | 10/10/10 | 1.16/1.28/1.27 |
| | | 1.4 | 20 | 1.75/1.70/1.72 | 10/10/20 | 1.27/1.27/1.29 |
| | | 1.0 | 40 | 1.11/1.06/1.06 | 10/10/10 | 0.98/0.92/0.97 |

[i]For datasets with multiple response variables, each row corresponds to a different response variable and the related dataset name is aligned with the first response variable.

[ii]RMSE values corresponding to the hyperparameter settings.

# Supplementary Figures

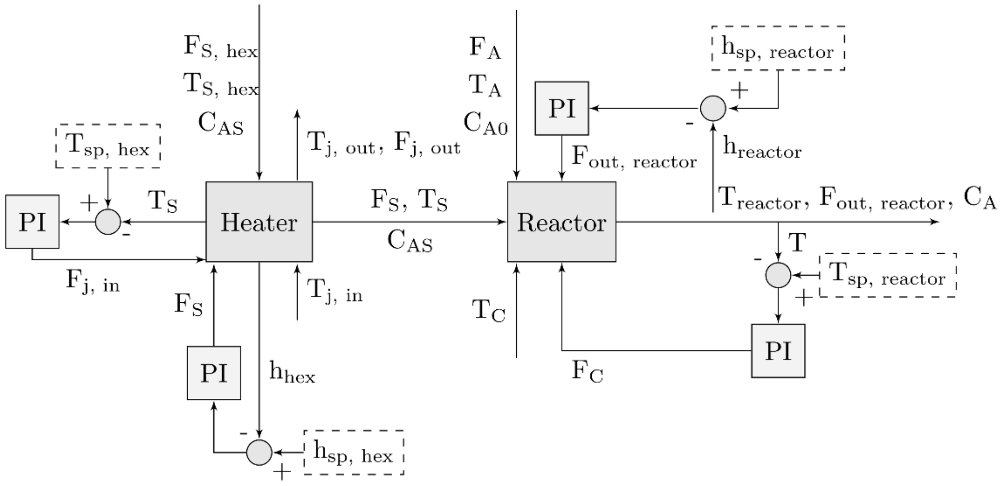


Fig. S1. Flow diagram of the reactor system simulated to generate the synthetic dataset.

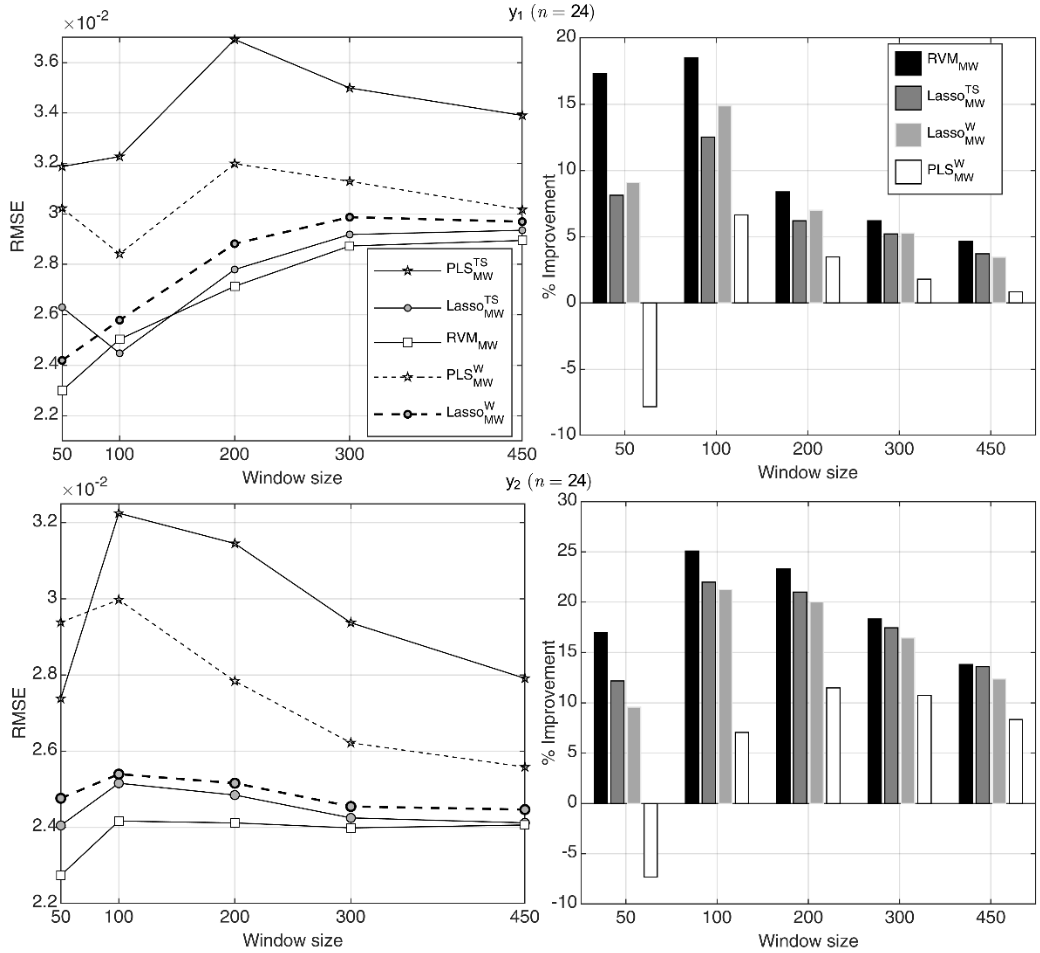


Fig. S2. Results of online learning experiments performed on Dataset 1 using $n$ = 24.

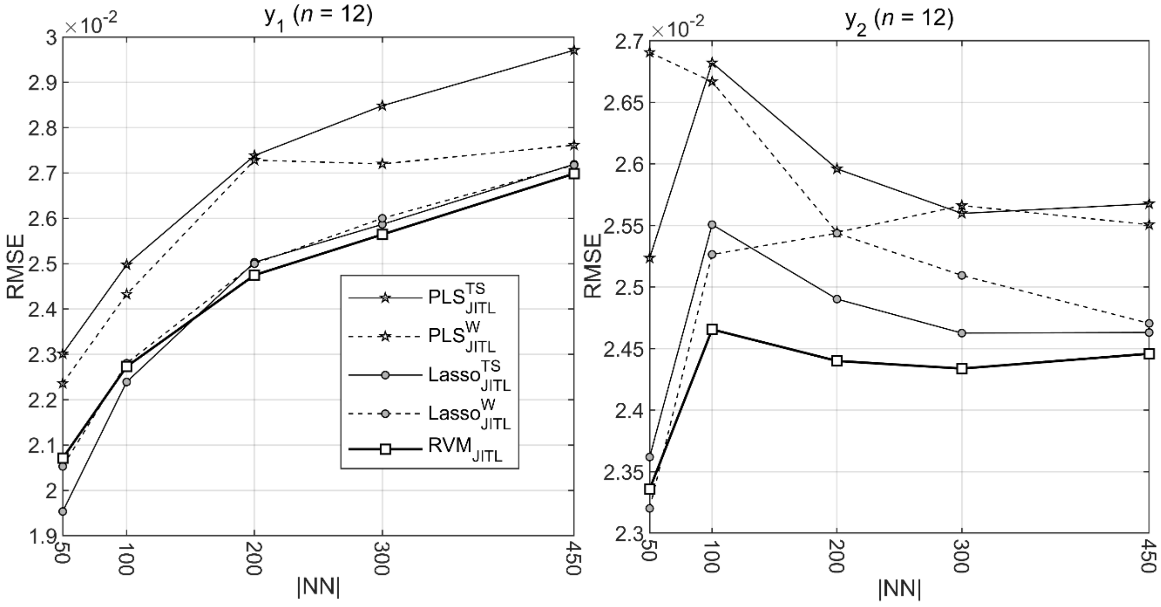


Fig. S3. Results of JITL method on Dataset 1 using $n$ = 12. |NN| represents the size of the training set comprised of nearest neighbors (NN).

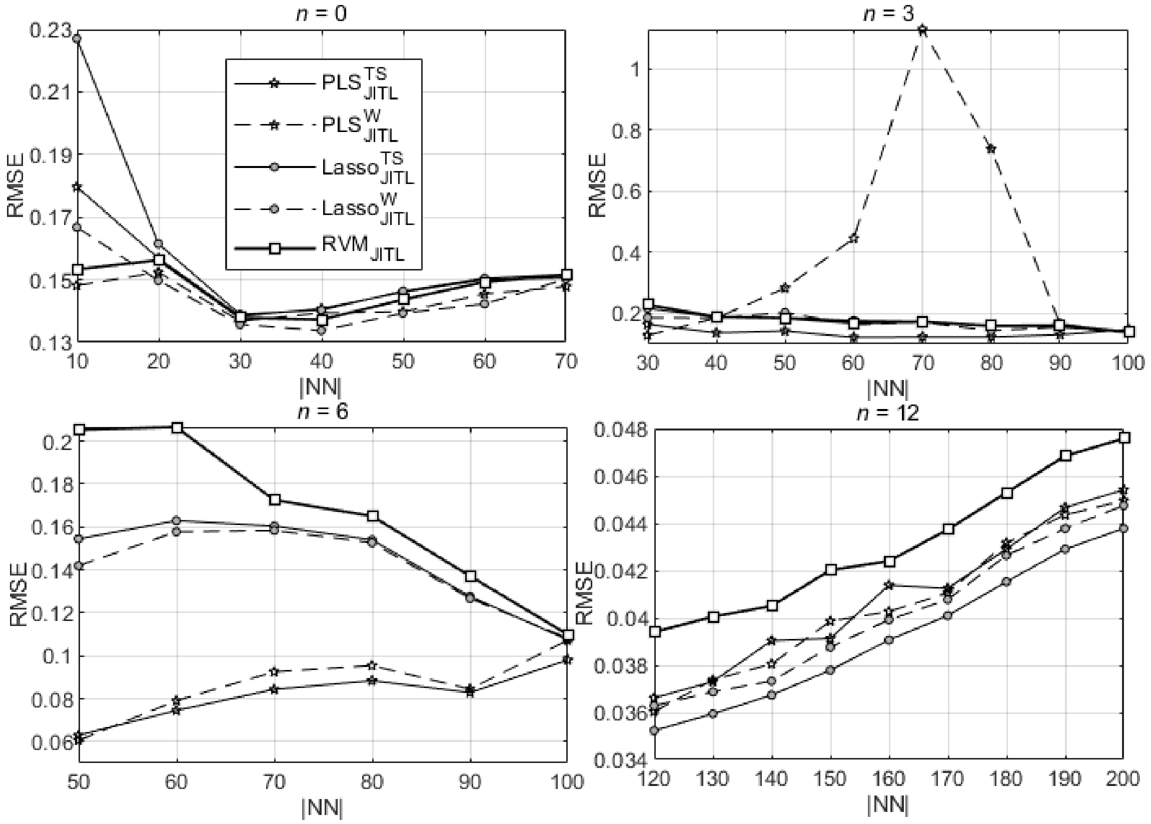


Fig. S4. Results of JITL method on Dataset 2.

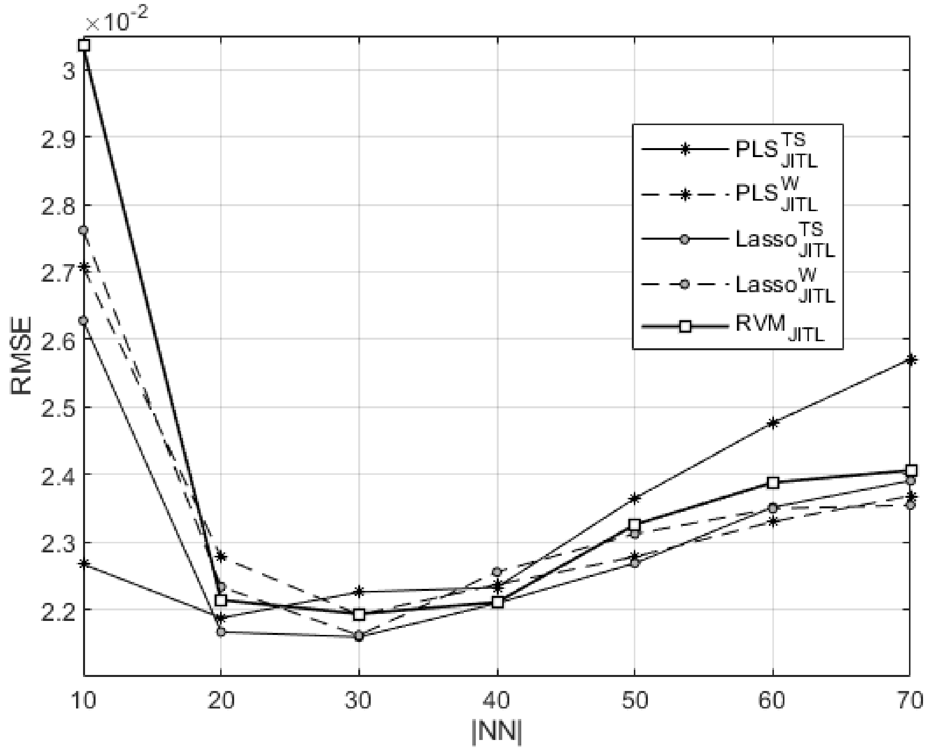


Fig. S5. Results of JITL method on Dataset 3.

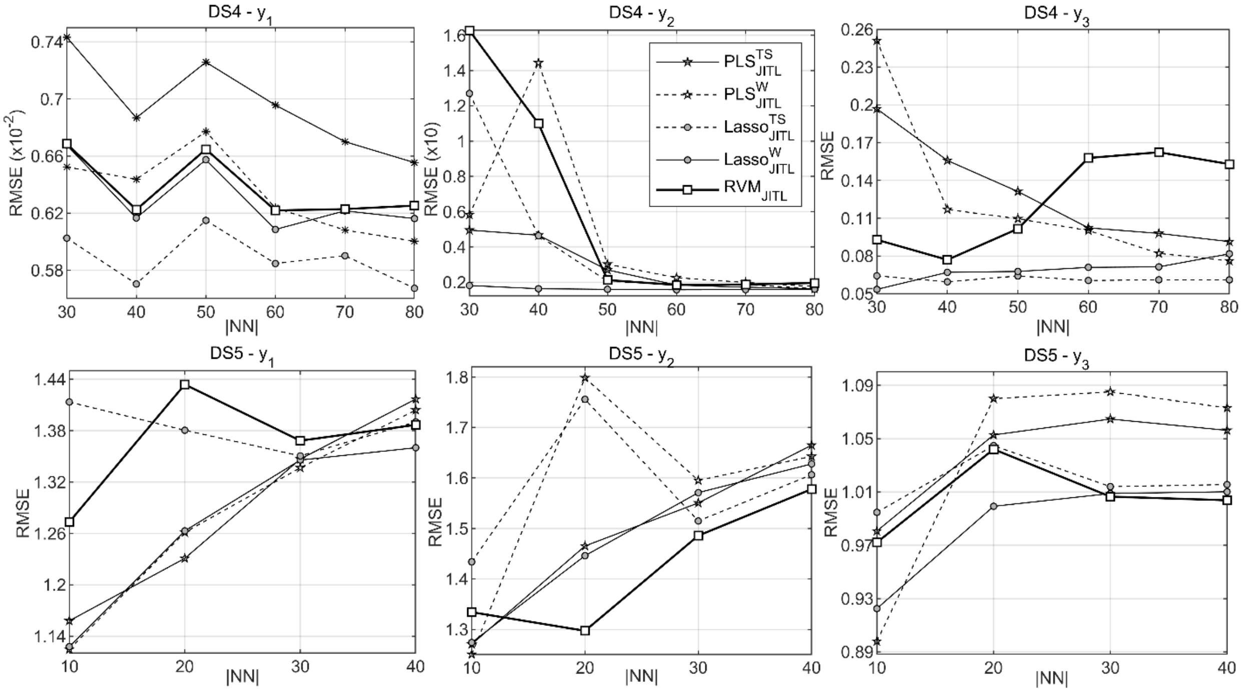


Fig. S6. Results of JITL method on Dataset 4 and Dataset 5.

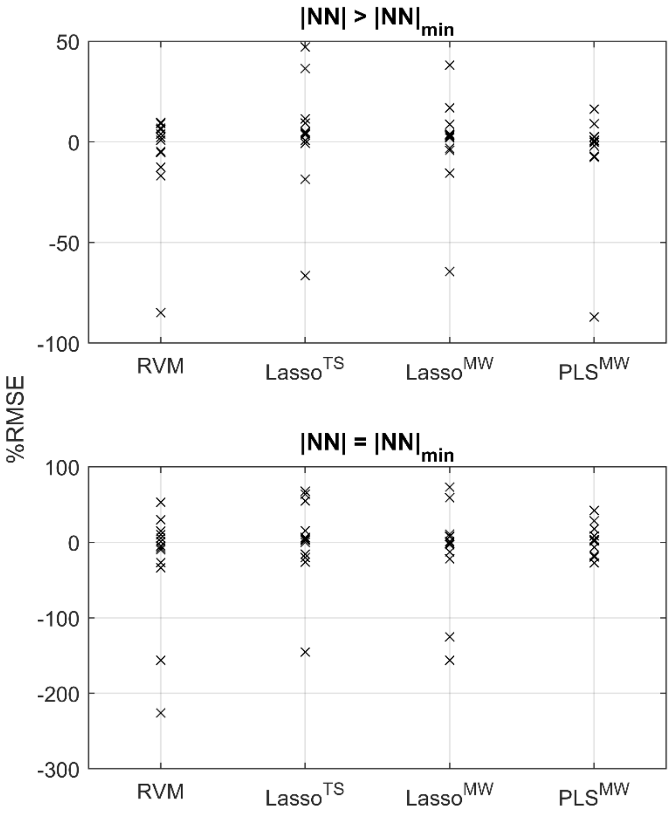


Fig. S7. Summary of %RMSE values for $|NN| > |NN|_{min}$ (top) and $|NN| = |NN|_{min}$ (bottom) with respect to learners under JITL scheme. Limits of the y-axis in the top figure adjusted to exclude a single sample of $PLS_{MW}^{W}$, which yields a %RMSE equal to -233%.
